# Supplementary material for: Optoelectronic excitations and photovoltaic effect in strongly correlated materials
Source: arXiv:1409.8261 source file (2014-09-29)
Supplement: Supplementary file 1 [file Coulter-Supplementary.pdf]

# Supplementary Material

## for the paper entitled

# Optoelectronic excitations and photovoltaic effect in strongly correlated materials

John E. Coulter
*Department of Physics and National High Magnetic Field Laboratory,*
*Florida State University, Tallahassee, FL 32306-4350, USA*

Efstratios Manousakis
*Department of Physics and National High Magnetic Field Laboratory,*
*Florida State University, Tallahassee, FL 32306-4350, USA and*
*Department of Physics, University of Athens, Panepistimioupolis, Zografos, 157 84 Athens, Greece.*

Adam Gali*
*Institute for Solid State Physics and Optics, Wigner Research Center for Physics,*
*Hungarian Academy of Sciences, Budapest, P.O.B. 49, H-1525 and*
*Department of Atomic Physics, Budapest University of Technology and Economics, Budafoki út 8., H-1111, Budapest, Hungary*
(Dated: September 3, 2014)

## I. STRUCTURE OF $VO_2$

The geometry of the most important phases of vanadium dioxide ($VO_2$) is briefly described here. The rutile phase is metallic where all the lattice vectors are perpendicular to each other. The insulating $M_1$ phase of $VO_2$ ($M_1$-$VO_2$) is a distorted structure where V1, V1' and V2, V2' as well as the corresponding oxygen atoms will be symmetrically inequivalent compared to the case of rutile phase. The "a" axis goes along the zig-zag distortion in $M_1$-$VO_2$. In plots concerning the optical properties, we refer to light polarized either parallel or perpendicular to this "a" axis.

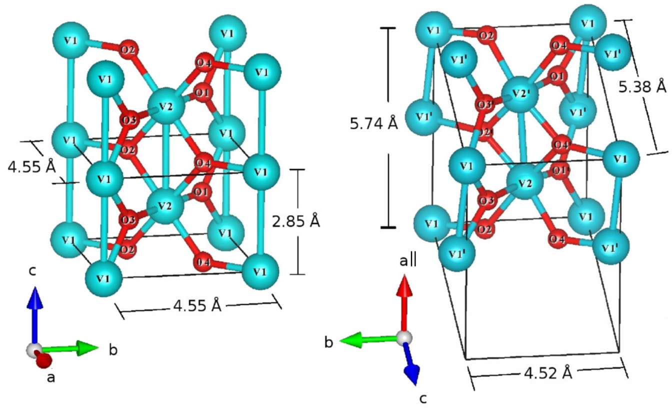


FIG. S1. Geometry of the rutile (left) $VO_2$ compared to the $M_1$ phase (right) of $VO_2$. The experimental lattice constants are given as well as the traditional labeling of the lattice vectors. The symmetrically equivalent atoms are labeled correspondingly.

## II. BAND STRUCTURE OF $VO_2$

Here we provide a brief description of the bands in $M_1$-$VO_2$, for reference in other discussion. The highest dispersion occurs along the $\Gamma$-$Z$ direction, which is the direction of the zig-zag distortion in the $M_1$-$VO_2$ lattice. The high dispersion along the $\Gamma$-$Y$ and $\Gamma$-$B$ directions occurs along the other two unit cell axes, between $V$ atoms.

## III. DETAILS ABOUT BSE CALCULATIONS

### A. Implementation of BSE

For the optical properties we solve the BSE by diagonalizing the well-known electron-hole pair Hamiltonian,[1]

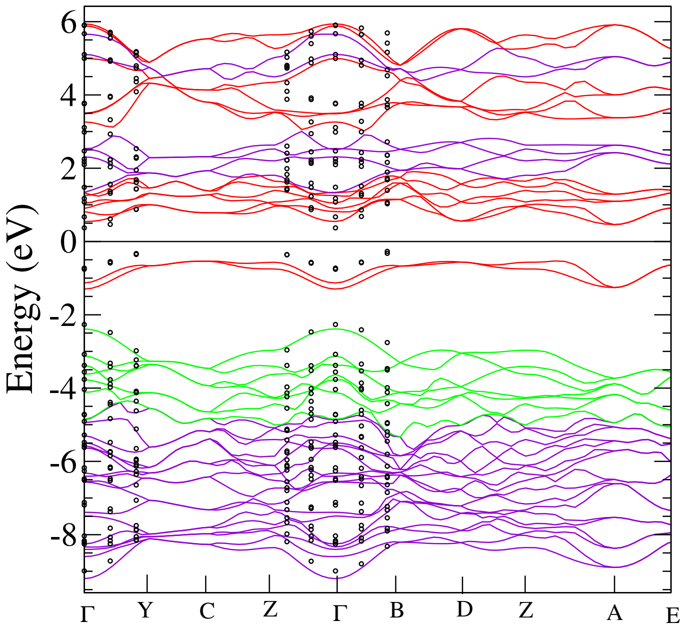


FIG. S2. The band structure of $M_1$-$VO_2$ calculated within HSE06 and HSE06+scGW. The bands with highly correlated electrons are shown with red colors, while simple p-type bands are shown in green, and mixed character bands are shown in violet. Bands from scGW are represented as points, as a full band-structure calculation is very expensive. The origin is set to the middle of the calculated band gap.

$$
\begin{aligned}
\omega A_{vc\mathbf{k}} &= (E_{c\mathbf{k}} - E_{v\mathbf{k}})\delta_{vv'}\delta_{cc'}\delta_{\mathbf{kk}'}A_{vc\mathbf{k}} + \\
&\sum_{v'c'} K^{AA}_{\substack{v'c'\mathbf{k}'\\ vc\mathbf{k}}}(\omega)A_{v'c'\mathbf{k}'} + \\
&\sum_{v'c'} K^{AB}_{\substack{v'c'\mathbf{k}'\\ vc\mathbf{k}}}(\omega)B_{v'c'\mathbf{k}'}, \\
-\omega B_{vc\mathbf{k}} &= (E_{c\mathbf{k}} - E_{v\mathbf{k}})\delta_{vv'}\delta_{cc'}\delta_{\mathbf{kk}'}B_{vc\mathbf{k}} + \\
&\sum_{v'c'} K^{BB}_{\substack{v'c'\mathbf{k}'\\ vc\mathbf{k}}}(\omega)B_{v'c'\mathbf{k}'} + \\
&\sum_{v'c'} K^{BA}_{\substack{vc\mathbf{k}\\ v'c'\mathbf{k}'}}(\omega)A_{v'c'\mathbf{k}'},
\end{aligned}
\tag{1}
$$

where the eigenenergies ($\omega$) of this Hamiltonian will provide the excitation energies whereas the eigenfunctions are the corresponding resonant and "antiresonant" two-particle exciton wave functions ($A_{vc\mathbf{k}}$ and $B_{vc\mathbf{k}}$). The diagonal form, $(E_{c\mathbf{k}} - E_{v\mathbf{k}})$ contains the quasi-particle energies as obtained from the GW approximation. The diagonal blocks of the BSE interaction kernel are the resonant part of $K^{AA}$ and the "antiresonant" part of $K^{BB}$, whereas $K^{AB}$ and $K^{BA}$ provide the off-diagonal blocks in the BSE matrix where the rank of the matrix depends on the number of valence $(v, v')$ bands $(n_v)$, conduction $(c, c')$ bands $(n_c)$, and k-points $(\mathbf{k}, \mathbf{k}')$ involved. The interaction matrix elements are written like (with $\mathbf{x} \equiv rt$):

$$
\begin{aligned}
K^{AA}_{\substack{vc\mathbf{k}\\ v'c'\mathbf{k}'}}(\omega) &= i\int d(3456)\psi_{v,\mathbf{k}}(\mathbf{x_4})\psi^*_{c,\mathbf{k}}(\mathbf{x_3})K(35,46;\omega) \\
&\qquad \times\psi^*_{v',\mathbf{k}'}(\mathbf{x_5})\psi_{c',\mathbf{k}'}(\mathbf{x_6}) \\
K^{AB}_{\substack{vc\mathbf{k}\\ v'c'\mathbf{k}'}}(\omega) &= i\int d(3456)\psi_{v,\mathbf{k}}(\mathbf{x_4})\psi^*_{c,\mathbf{k}}(\mathbf{x_3})K(35,46;\omega) \\
&\qquad \times\psi^*_{v',\mathbf{k}'}(\mathbf{x_6})\psi_{c',\mathbf{k}'}(\mathbf{x_5})
\end{aligned}
\tag{2}
$$

The structure of $K^{BB}$ and $K^{BA}$ is similar. The electron-hole interaction kernel $K(35, 46)$ consists of a "direct" and an "exchange" term, which involve the unscreened ($v$) and statically screened Coulomb interaction ($W$), respectively, in the form of $K = 2W - v$. We considered the coupling term $K^{AB}$ between the resonant and "antiresonant" states in our calculations. The valence and conduction band states are provided from the *scGW* procedure. The absorption spectrum can be calculated using $\omega$ and $A_{vc\mathbf{k}}$ where the individual absorption peaks appear around the poles ($\omega$).[2] Around the poles a small smearing constant is introduced which *influences* the intensity of the peaks. The choice of this smearing constant is arbitrary but, physically, it has a relation to the lifetime of excitons. As the BSE Hamiltonian in Eq. 1 provides real eigenvalues, the lifetime of excitons is not determined. That is a very complicated issue as the electron-phonon interaction plays an important role in the decay of excitons. The study of electron-phonon interaction in $M_1$-$VO_2$ is beyond the scope of this paper. A rational choice of the smearing constant is in the region of 0.05-0.15 $eV$.

## B. Testing the implementation of BSE on Si

We first tested the implementation of the BSE method against the absorption spectrum of silicon which is well known experimentally[3] and has been cross-checked by several theoretician research groups applying independent codes (see the most recent one in Ref. 4 and references therein). We used the experimental lattice constant of silicon crystal (5.43 Å), and a 12×12×12 $k$-point set[5], including all the valence bands and 8 conduction bands in the BSE equations. We find excellent agreement with experimental data, and, in fact, improve on other calculations in that regard (see Fig. S3). We attribute this improvement to the self-consistent GW methodology which provides a better description of the quasi-particle states. The excellent results here give us confidence that the implementation is correct, and that our results on the oxide materials will have no shortcomings other than those intrinsic to the BSE-method itself.

## C. Convergence of BSE on $M_1$-$VO_2$

The BSE calculation is computationally demanding because of the fact that one has to include the interac-

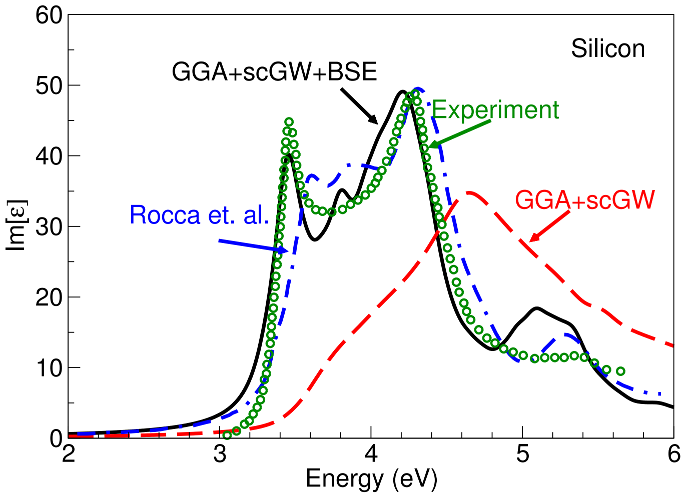


FIG. S3. The imaginary dielectric constant for Si within PBE+scGW+BSE. The calculated results agree well with the experimental data in Ref. 3, and similar GW+BSE results have been published by others (see Rocca *et al.* study in Ref. 4 and references therein). We conclude that the implementation of the BSE method that we used produces correct results.

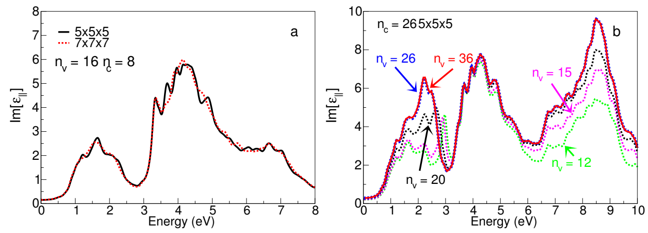


FIG. S4. (a) The parallel to the $a$-axis imaginary part of the dielectric function as calculated for a 5×5×5 and a 7×7×7 $k$-point set where $n_v$=18 and $n_c$=8. (b) Convergence of $\epsilon_{2||}$ with number of valence bands ($n_v$) using a fixed number of conduction bands ($n_c$) for the case of the full BSE calculation. All calculations here use HSE06+$G_0W_0$+BSE.

tion of electron-hole pairs with different relative momenta and from different bands. The primitive cell of Si crystal contains only two atoms, and four valence electrons per atom, and has a high $O_h$ symmetry. This makes it possible to easily achieve fully convergent results for crystalline Si. However, the primitive cell of $M_1$-$VO_2$ contains 8 oxygen and 4 vanadium atoms with six and eleven valence electrons, respectively, and the symmetry of the crystal is much lower than for Si, meaning that many fewer k-points are symmetrically equivalent in its Brillouin-zone. As a consequence, to make the calculation feasible within a realistic computational time scale, we need to limit the $k$-point size and the number of bands involved in the BSE kernel for $M_1$-$VO_2$.

We studied the convergence with respect to the size of $k$-point set used in our calculations. In the convergence tests HSE06+$G_0W_0$+BSE is used, as doing convergence tests on top of the scGW calculation was too computationally expensive, where $G_0W_0$ means the single shot GW-method. Since the HSE06+$G_0W_0$ provided qualitatively good results[6] the conclusions basically holds for DFT+scGW based BSE calculations. In Fig. S4(a) we compare our calculated imaginary part of the dielectric function $\epsilon_2$ parallel to the $a$-axis ($\epsilon_{2||}$) for a 5×5×5 and a 7×7×7 $k$-point set[5], by including the same number of valence and conduction bands in both calculations. Notice that the results of these two calculations agree reasonably well and, thus, we have adopted the 5 × 5 × 5 $k$-point set in the full DFT+scGW+BSE calculation. We note that this $k$-point set may not be fully convergent, however, one can not afford much more with a full diagonalization of the BSE matrix even on a very high performance computer cluster. We note that the bands are relatively flat in many directions in the Brillouin-zone (see Fig. S2), which can explain the relatively fast convergence in the calculated optical spectra. In $a$-direction (parallel direction) this convergence may be slower as the dispersion of bands is larger than that in perpendicular directions.[6] Nevertheless, this choice of $k$-point set seems to provide reasonable a spectrum.

In Fig. S4(b) we demonstrate that using $n_v$=26 may be sufficient to achieve a satisfactory level of accuracy for $\epsilon_{2||}$ as these results are very close to those obtained for $n_v$ = 36. In all the calculations presented in Fig. S4(b), we have used $n_c$=26. We have also studied the convergence with respect to the number of the conduction bands by keeping the number of valence bands fixed and found that when $n_c$ = 26, the results have converged. Therefore, all the results presented in this paper are obtained with $n_v$=$n_c$=26 that provide convergent results in the low-energy excitation spectrum, including the onset of absorption that is relevant in the solar spectrum. A smearing parameter of 0.1 eV is applied. We emphasize that the total calculation time was 0.5 million of CPU hours on supercomputers even with these limitations of $k$-point set and the number of states.

## IV. COMPARISON OF PREVIOUS THEORETICAL WORK ON THE IIR IN SI

Our main focus in our paper is to show that the IIR can be *higher* than $10^{12}$-$10^{13}$ $s^{-1}$ in the energy range of the solar spectrum for strongly correlated materials. As explained in the Methods section of the main text, we estimated the IIR from the imaginary part of the calculated self-energy within GW theory. The implementation of GW and the self-energy calculation within the applied code is described in detail in Ref. 7. The polarizability function (needed to calculate the GW self-energy) is calculated on a frequency grid. We found that the IIR is sensitive to the density of this grid. The energy grid is non-linear, and optimized for the spectral integrals used in the current implementation. There is a built-in smear-

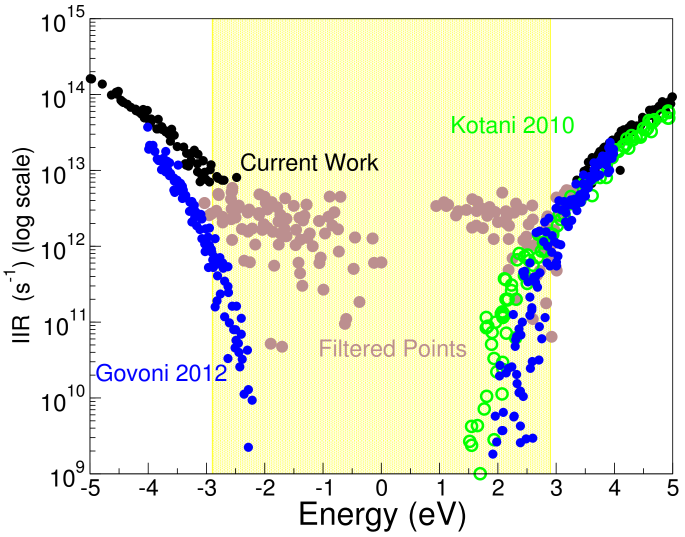


FIG. S5. Estimated impact ionization rate (IIR) as a function of excitation energy in silicon. The electron and hole-initiated biexcitons were both considered. Our results are compared to previous calculations by Govoni *et al.*, Kotani *et al.* in Refs. 8 and 9. Kotani *et al.* applied the same approximation in the self-energy that we do, though a different basis set was used. Areas in our calculation which are numerically inaccurate are shown in grey. We also highlight (yellow) the energy regions in which bi-excitons can be created by light in the solar spectrum.

ing due to the grid density, coming from the treatment of the energy-conserving delta function in the spectral function[7]. This grid is the current obstacle to improving the accuracy of our calculation, as we are limited by the amount of computer memory available. We currently use a grid spacing of 0.02 eV at the lowest energies, which leads to the imaginary self energy converged to within 0.002 eV in the region of interest. This corresponds to an IIR of 6x10$^{12}$ $s^{-1}$. Since impact ionization with IIR below 6x10$^{12}$ s$^{-1}$ is not competitive with the process of phonon decay we did not aim to accurately calculate very low IIR values. Thus, we do not show those values in Fig. 4 in the main text that should go below the threshold of 6x10$^{12}$ s$^{-1}$. We emphasize that the IIR values higher than that threshold are convergent. In order to illustrate this, we compare our calculated data and previous results from independent codes and sources on Si in Fig. S5.

The values in Si are well-reproduced for those excitation energy regions where the IIR has about the same order of magnitude as the rate of phonon decay, and excellent agreement is achieved for those energy regions where IIR outcompetes the rate of the decay of phonons.

In $VO_2$, we are able to converge the self-energy to within 0.03 eV, which means our results are truncated above a rate of 6x10$^{13}$ $s^{-1}$. Again, this does not change our conclusions at all. It is extremely difficult to increase the accuracy in $VO_2$. Due to the complicated structure and large number of electrons, it takes a large amount of time and memory, even for a high-performance cluster.

* gali.adam@wigner.mta.hu

[1] Rohlfing, M. & Louie, S. G. Electron-hole excitations and optical spectra from first principles. *Phys. Rev. B* **62**, 4927–4944 (2000). URL http://link.aps.org/doi/10.1103/PhysRevB.62.4927.

[2] Onida, G., Reining, L. & Rubio, A. Electronic excitations: density-functional versus many-body green's-function approaches. *Rev. Mod. Phys.* **74**, 601–659 (2002). URL http://link.aps.org/doi/10.1103/RevModPhys.74.601.

[3] Lautenschlager, P., Garriga, M., Vina, L. & Cardona, M. Temperature dependence of the dielectric function and interband critical points in silicon. *Phys. Rev. B* **36**, 4821–4830 (1987).

[4] Rocca, D., Ping, Y., Gebauer, R. & Galli, G. Solution of the bethe-salpeter equation without empty electronic states: Application to the absorption spectra of bulk systems. *Phys. Rev. B* **85**, 045116 (2012). URL http://link.aps.org/doi/10.1103/PhysRevB.85.045116.

[5] Monkhorst, H. J. & Pack, J. D. Special points for brillouin-zone integrations. *Phys. Rev. B* **13**, 5188–5192 (1976).

[6] Coulter, J. E., Manousakis, E. & Gali, A. Limitations of the hybrid functional approach to electronic structure of transition metal oxides. *Phys. Rev. B* **88**, 041107 (2013). URL http://link.aps.org/doi/10.1103/PhysRevB.88.041107.

[7] Shishkin, M. & Kresse, G. Implementation and performance of the frequency-dependent *gw* method within the paw framework. *Phys. Rev. B* **74**, 035101 (2006).

[8] Govoni, M., Marri, I. & Ossicini, S. Carrier multiplication between interacting nanocrystals for fostering silicon-based photovoltaics. *Nature Photonics* **6**, 672–679 (2012).

[9] Kotani, T. & van Schilfgaarde, M. Impact ionization rates for si, gaas, inas, zns, and gan in the *gw* approximation. *Phys. Rev. B* **81**, 125201 (2010). URL http://link.aps.org/doi/10.1103/PhysRevB.81.125201.
